# Supplementary material for: The Abrikosov vortex structure revealed through near-field radiative heat exchange
Source: arXiv:2306.01228 source file (2023-06-02)
Supplement: Supplementary file 1 [file supplementary_230523_SGCL.pdf]

# Supplementary Information.
# The Abrikosov vortex structure revealed through near-field radiative heat exchange.

S. G. Castillo-López, R. Esquivel-Sirvent, G. Pirruccio, C. Villarreal*
*Instituto de Física, Universidad Nacional Autónoma de México, Cd. de México C.P. 04510 Mexico.*
(Dated: May 30, 2023)

## TEMPERATURE DEPENDENCE OF VORTEX LATTICE PERIODICITY

The order parameter forms a periodic lattice of vortexes with spatial periods, $\mathcal{L}_x = \mathcal{L}_y = \sqrt{2\pi}\xi(T)$, where $\xi^2(T) = \xi^2(0)/(1 - T^2/T_c^2)$ for finite temperatures. Experimental observations suggest that the zero temperature coherence length in YBCO, $\xi_0 \sim 1.6$ nm, so that the lattice periodicity has the temperature dependence shown in Fig. S1.

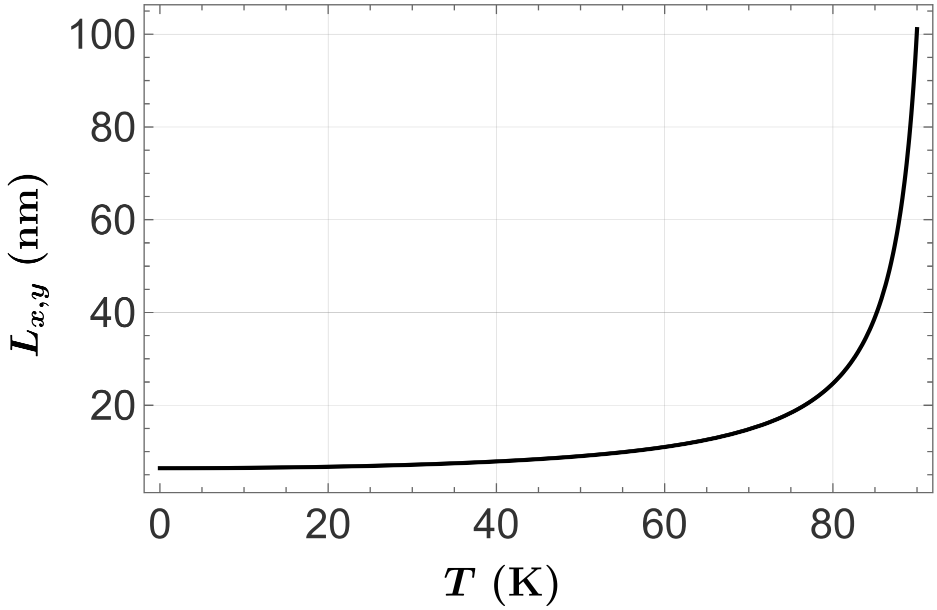


Fig. S 1: Temperature dependence of the lattice parameter $\mathcal{L}_{x,y}$ in the Abrikosov vortex structure.

## DIELECTRIC RESPONSE OF YBCO

The dielectric response of YBCO along the *ab*-planes may be represented in the normal phase, $T \geq T_c$, as a superposition of Lorentz-type dielectric functions, Drude, mid-infrared (MIR), and phonon contributions [1, 2]:

$$\varepsilon_{ab}^{(n)}(\omega, T) = \varepsilon_\infty - \frac{\omega_p^2}{\omega^2 + i\gamma(T)\,\omega} - \frac{\Omega_{mir}^2}{\omega^2 - \omega_{mir}^2 + i\Gamma_{mir}\,\omega} - \sum_{k=1}^{Nph} \frac{\Omega_{ph,k}^2}{\omega^2 - \omega_{k,ph}^2 + i\gamma_{k,ph}\,\omega}, \tag{S1}$$

In the SC phase, $T < T_c$, dissipative scattering does not occur, so that $\gamma(T) \to 0$, and the dielectric response becomes:

$$\varepsilon_{ab}^{(s)}(\omega, \mathbf{r}, T) = \varepsilon_\infty - \frac{\omega_p^2}{\omega^2}\left(1 - \frac{T^2}{T_c^2}\right)|\Psi_0(\mathbf{r})|^2\left[1 + \frac{i\pi\omega\delta(\omega)}{2}\right] - \left(\frac{T^2}{T_c^2}\right)\frac{\omega_p^2}{\omega^2 + i\gamma'(T)\,\omega} - \frac{\Omega_{mir}^2}{\omega^2 - \omega_{mir}^2 + i\gamma_{mir}\,\omega} - \sum_{k=1}^{Nph}\frac{\Omega_{ph,k}^2}{\omega^2 - \omega_{k,ph}^2 + i\gamma_{k,ph}\,\omega} \tag{1}$$

In the former expressions, $\omega_p(100\text{ K}) = 0.75$ eV, $\gamma(T) = \gamma_0 + \beta T$ eV, with $\gamma_0 = 0.03$, and $\beta = 8\times10^{-5}$, and $\gamma' = \gamma(T_c)$. The rest of parameters is identical in both expressions: $\varepsilon_\infty = 3.8$, $\Omega_{mir} = 2.6$ eV, $\omega_{mir} = 0.26$ eV, $\Gamma_{mir} = 1$ eV, whereas the phonon contributions are reported in Ref.([1, 2]).

## NEAR-FIELD HEAT TRANSFER CALCULATION

In the near-field, the spectral heat flux is calculated from Rytov's theory of fluctuating electrodynamics [3] as

$$S_\omega(\omega, T_{ns}, T_{sub}, L, \mathbf{r}_\perp) = [\Theta(\omega, T_{ns}) - \Theta(\omega, T_{sub})]\,[\rho_\omega^{prop}(\mathbf{r}, L, T) + \rho_\omega^{evan}(\mathbf{r}, L, T)]\,, \tag{S3}$$

where $\rho_{prop}$ and $\rho_{evan}$ represent the density of the propagating ($\omega/c > \kappa$) and evanescent ($\omega/c < \kappa$) modes, respectively. For the setup concerning our paper:

$$\rho_\omega^{prop} = \frac{\omega^2}{c^2}\int \frac{d^3\kappa}{(2\pi)^3}\frac{2}{k_{z0}}\alpha''_{ns}(\omega, T_{ns})\sum_{i=s,p}\left[1 - |r_i(\omega, \kappa, T_{sub}, \mathbf{r}_\perp)|^2\right], \tag{S4}$$

$$\rho_\omega^{evan} = \frac{\omega^2}{c^2}\int \frac{d^3\kappa}{(2\pi)^3}\frac{4e^{-2\gamma L}}{\gamma}[\alpha''_{ns}(\omega, T_{ns})]\Big\{r''_s(\omega, \kappa, T_{sub}, \mathbf{r}_\perp) + \left[\frac{2\kappa^2}{(\omega/c)^2} - 1\right] r''_p(\omega, \kappa.T_{sub}, \mathbf{r}_\perp)\Big\}. \tag{S5}$$

Here, $\Theta(\omega, T) = \hbar\omega/[\exp(\hbar\omega/k_B T) - 1]$ is the Planckian distribution, and $\kappa$ is the component of the wavevector parallel to the substrate interface. Within the dipolar approximation, the nanosphere polarizability, $\alpha_{ns} = 4\pi R^3(\varepsilon_{ns}(\omega, T_{ns}) - 1)/(\varepsilon_{ns}(\omega, T_{ns}) + 2)$; and the Fresnel reflection coefficients are,

$$r_s = \frac{k_{z0} - k_z}{k_{z0} + k_z}, \qquad r_p = \frac{\varepsilon_{sub}\, k_{z0} - k_z}{\varepsilon_{sub}\, k_{z0} + k_z}. \tag{S6}$$

with $k_{z0} = \sqrt{(\omega/c)^2 - \kappa^2} = i\gamma$, $k_z = \sqrt{\varepsilon_{sub}(\omega, \mathbf{r}_\perp)\,(\omega/c)^2 - \kappa^2}$; $\varepsilon_{sub}(\omega, \mathbf{r}_\perp, T_{sub}) = \varepsilon_{ab}^{(s)}(\omega, \mathbf{r}_\perp, T_{sub})$ and $\varepsilon_{ns}(\omega, T_{ns}) = \varepsilon_{ab}^{(n)}(\omega, T_{ns})$ represent the substrate and nanosphere permittivity, respectively.

## CONTRIBUTION OF SURFACE MODES TO SPECTRAL HEAT FLUX

Along the Abrikosov vortexes lattice exhibited by the YBCO substrate, surface modes (SMs) are selectively excited in certain regions of the lattice at specific frequencies ($\omega_i$), where the condition $\varepsilon_{ab}^{(s)}(\omega_i) = -1$ is satisfied. Fig. S2 shows the Re and Im parts of the dielectric function $\varepsilon_{ab}^{(s)}(\omega)$ at the positions (a) $x = 0.5\mathcal{L}_x,\ y = 0.5\mathcal{L}_y$ and (b) $x = 0.5\mathcal{L}_x,\ y = 0.4\mathcal{L}_y$ on the Abrikosov lattice. The vertical dashed lines indicate the frequencies $\omega_i$ in each case. In Figs. S2 (c) and (d), we plot the spectral heat flux $S_\omega(y)$ along the $y$ direction for the specific frequencies $\omega_i$ corresponding to Fig. S2 (a) and (b). In both cases, the largest modulation of $S_\omega(y)$ is observed with the first resonance frequency $\omega_1$. The other curves show a smaller modulation due to the high damping of the modes at these frequencies, characterized by high values of $\mathrm{Im}\varepsilon_{ab}^{(s)}(\omega)$.

---

* Also at


[1] S. Castillo-López, G. Pirruccio, C. Villarreal, and R. Esquivel-Sirvent, Sci. Rep. **10**, 16066 (2020).
[2] S. Castillo-López, C. Villarreal, R. Esquivel-Sirvent, and G. Pirruccio, International Journal of Heat and Mass Transfer **182**, 121922 (2022).
[3] E. A. Vinogradov and I. A. Dorofeev, Physics-Uspekhi **52**, 425 (2009).

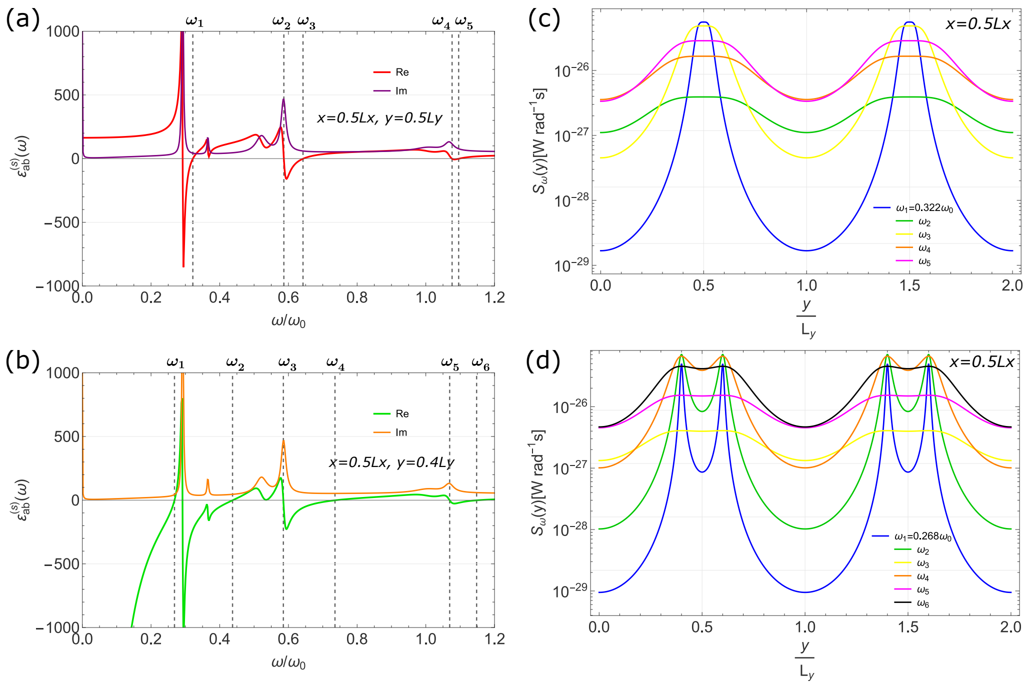


Fig. S 2: Real and imaginary parts of YBCO permittivity $\varepsilon_{ab}^{(s)}(\omega, 2K)$ as a function of the normalized frequency $\omega/\omega_0$ at the position (a) $x = 0.5\mathcal{L}_x,\ y = 0.5\mathcal{L}_y$ and (b) $x = 0.5\mathcal{L}_x,\ y = 0.4\mathcal{L}_y$ in the Abrikosov lattice. Vertical dashed lines indicate the frequencies $\omega_i$ where the SM excitation condition is met, $\varepsilon_{ab}^{(s)}(\omega_i) = -1$. Spatial dependence of the heat flux $S_\omega(y)$ for the different values of $\omega_i$ corresponding to (c) Fig. (a), and (d) Fig.(b). Here $x = 0.5\mathcal{L}_x$, $T_{ns} = 300$ K, and $T_{sub} = 2$ K.
